# Supplementary material for: Learning for Bandits under Action Erasures
Source: arXiv:2406.18072 source file (2024-06-26)
Supplement: Supplementary file 1 [file appendix.tex]

\section{LINEAR PROGRAM FORMULATION}
\label{app:lp-formulation}
We first formulate a (nonlinear integer) program  that minimizes the end time to schedule action pulls in batch $i$ with $K$ actions across $M$ agents as follows:
\begin{subequations}
\label{p:formulation}
\begin{empheq}[box=\widefbox]{align}
    \min\limits_{\mX \in \mathbb{R}^{M \times K} } &~~ \max\limits_{m \in [M]} \sum\limits_{k=1}^{K} \left( \alpha_m \mathds{1}[X_{mk} > 0] + X_{mk} \right) \label{p:objective}\\
    \text{s.t.} ~~&~~  \sum\limits_{m=1}^{M} X_{mk} = 4^i ~~~\forall k \in [K] \label{p:sum}\\
    &~~  X_{mk} \in \{0,1,2,\cdots,4^i \} ~~~\forall m \in [M], ~\forall k \in [K] \label{p:integer},
\end{empheq}
\end{subequations}where $\mX \in \mathbb{R}^{M \times K}$ captures the variables of the program, with $X_{mk}$ indicating the number of effective pulls of action $k$ performed by agent $m$. The objective function (\ref{p:objective}) is to minimize the latest end time among agents. Constraint ($\ref{p:sum}$) ensures that the total number of effective pulls for each action is $4^i$; and constraint (\ref{p:integer}) forces effective pulls assigned to each agent per action to be an integral value in $[0,4^i]$. It is easy to see that the progam in (\ref{p:formulation}) is equivalent to the following  integer linear program (ILP): 
\begin{subequations}
\label{ilp:formulation}
\begin{empheq}[box=\widefbox]{align}
    \min\limits_{\substack{\mX, \mW \in \mathbb{R}^{M \times K} \\  t \in \mathbb{R} }} &~~~~ t \label{ilp:objective}\\
    \text{s.t.} ~~~~~&~~ \sum\limits_{k=1}^{K} \left( \alpha_m W_{mk} + X_{mk} \right) \leq t,  ~~~\forall m \in [M] \label{ilp:obj_to_const}\\
    &~~ X_{mk} \leq 4^i W_{mk} ~~~\forall m \in [M], ~\forall k \in [K] \label{ilp:indicator}\\
    &~~  \sum\limits_{m=1}^{M} X_{mk} = 4^i ~~~\forall k \in [K] \label{ilp:sum}\\
    &~~  X_{mk} \in \{0,1,2,\cdots,4^i \} ~~~\forall m \in [M], ~\forall k \in [K] \label{ilp:integer_x} \\
    &~~  W_{mk} \in \{0,1 \} ~~~\forall m \in [M], ~\forall k \in [K] \label{ilp:integer_w},
\end{empheq}
\end{subequations} where the variable $t \in \mathbb{R}$ replaces the $\max$ in objective \eqref{p:objective} and the variable $\mW \in \mathbb{R}^{M \times K}$ replaces the indicator function. Notice that for any feasible solution $\mX$, if $X_{mk} > 0$, $W_{mk} = 1$. The relaxed version of the ILP in (\ref{ilp:formulation}) can be written as 

\begin{subequations}
\label{lp:relaxed_formulation}
\begin{empheq}[box=\widefbox]{align}
    \min\limits_{\substack{\mX, \mW \in \mathbb{R}^{M \times K} \\  t \in \mathbb{R} }} &~~~~ t \label{lp:relaxed_objective}\\
    \text{s.t.} ~~~~~&~~ \sum\limits_{k=1}^{K} \left( \alpha_m W_{mk} + X_{mk} \right) \leq t,  ~~~\forall m \in [M] \label{lp:relaxed_obj_to_const}\\
    &~~ \mX_{mk} \leq 4^i W_{mk} ~~~\forall m \in [M], ~\forall k \in [K] \label{lp:relaxed_indicator}\\
    &~~  \sum\limits_{m=1}^{M} X_{mk} = 4^i ~~~\forall k \in [K] \label{lp:relaxed_sum}\\
    &~~  0 \leq X_{mk} \leq 4^i ~~~\forall m \in [M], ~\forall k \in [K] \label{lp:relaxed_integer_x} \\
    &~~ 0 \leq W_{mk} \leq 1 ~~~\forall m \in [M], ~\forall k \in [K] \label{lp:relaxed_integer_w},
\end{empheq}
\end{subequations}

Notice that the minimum value $W_{mk}$ can take is $X_{mk} / 4^i$ due to (\ref{lp:relaxed_indicator}); hence, by replacing $W_{mk}$ with its minimum value, we get the following linear program which gives a lower bound on the ILP (\ref{ilp:formulation}):

\begin{subequations}
\label{lp:formulation}
\begin{empheq}[box=\widefbox]{align}
    \min\limits_{\substack{\mX \in \mathbb{R}^{M \times K} \\  t \in \mathbb{R} }} &~~~~ t \label{lp:objective}\\
    \text{s.t.} ~~~~~&~~ \sum\limits_{k=1}^{K} X_{mk} \left(  \frac{\alpha_m}{4^i}  + 1 \right) \leq t  ~~~\forall m \in [M] \label{lp:obj_to_const}\\
    &~~  \sum\limits_{m=1}^{M} X_{mk} = 4^i ~~~\forall k \in [K] \label{lp:sum}\\
    &~~  0 \leq X_{mk} ~~~\forall m \in [M], ~\forall k \in [K] \label{lp:nonneg_x},
\end{empheq}
\end{subequations}
In the linear program (\ref{lp:formulation}), $X_{mk}$ is the variable that indicates how many effective pulls are assigned to agent $m$ for action $k$. (\ref{lp:sum}) forces each action to be pulled $4^i$ effective times; however, instead of an integer number of pulls, each agent is allowed to perform nonnegative fractional pulls. Furthermore, (\ref{lp:obj_to_const}) indicates that for each agent $m$, one effective pull has a cost of $\frac{\alpha_m}{4^i} + 1$.

\begin{claim}\label{claim:optimal_soln_lp}
    The optimal objective value of (\ref{lp:formulation}) satisfies, $t^\star = \sum_{k=1}^{K} X_{mk}^\star (\alpha_m / 4^i + 1) ~\forall m \in M$, where ($t^\star, \mX^\star$) is the optimal solution of \ref{lp:formulation}.
    %$t^\star = \frac{K 4^i}{\sum_{m=1}^{M} 1 / (\alpha_m/4^i + 1)}$.
\end{claim}

\noindent{\textit{Proof of Claim~\ref{claim:optimal_soln_lp}.}
First, we observe that at least one of the inequalities in (\ref{lp:obj_to_const}) holds with equality, otherwise the value of $t^\star$ can be decreased leading to a better objective. Define the set of indices $\gE_i := \{m \in [M] : \sum_{k=1}^{K} X_{mk}^\star (\alpha_m / 4^i + 1) = t^\star\}$.

Now, assume Claim~\ref{claim:optimal_soln_lp} is not correct. And let $m_s$ be such that$$\sum_{k=1}^{K} X_{m_sk}^\star (\alpha_{m_s} / 4^i + 1) < t^\star.$$
Then $\forall m \in \gE_i ~\exists \{ \beta_{mk} \}_{k=1}^{K} \geq 0: \sum_k \beta_{mk} > 0 $ small enough such that 
\ifarxivFormat
\begin{align}
    &X'_{mk} = \begin{cases}
        X^\star_{mk} - \beta_{mk}, & m \in \gE_i,~\forall k \in [K] \\
        X^\star_{m k} + \sum_{k=1}^{K} \beta_{mk} , &~ m_s = m \\
        X^\star_{mk} &~ \text{otherwise}
    \end{cases} \nonumber \\
    &t' = \max_{m} \{ \sum_{k=1}^{K} X_{mk}^{'} (\alpha_m / 4^i + 1) \} < t^\star \nonumber
\end{align}
\else
\begin{align}
    &X'_{mk} = \begin{cases}
        X^\star_{mk} - \beta_{mk}, & m \in \gE_i,~\forall k \in [K] \\
        X^\star_{m k} + \sum_{k=1}^{K} \beta_{mk} , &~ m_s = m \\
        X^\star_{mk} &~ \text{otherwise}
    \end{cases} \nonumber \\
    &t' = \max_{m} \{ \sum_{k=1}^{K} X_{mk}^{'} (\alpha_m / 4^i + 1) \} < t^\star \nonumber
\end{align}
\fi
forms a feasible solution in (\ref{lp:formulation}) with a smaller objective value $t' < t^\star$; hence, $(t^\star, \mX^\star)$ cannot be optimal. Then at the optimal solution $(t^\star, \mX^\star)$, $t^\star = \sum_{k=1}^{K} X_{mk}^\star (\alpha_m / 4^i + 1) ~\forall m \in M$.

Using Claim~\ref{claim:optimal_soln_lp} and the constraint (\ref{lp:sum});\ifarxivFormat\begin{align}\label{t_star}
    4^i K = \sum_{m=1}^{M} \sum_{k=1}^{K} X^\star_{mk} = \sum_{m=1}^{M} \frac{t^\star}{ (\alpha_m/4^i + 1)} ~=~ t^\star \sum_{m=1}^{M} \frac{1}{(\alpha_m/4^i + 1) } \nonumber \\
    ~\Rightarrow~~ t^\star ~=~ \frac{4^i K}{\sum_{m=1}^{M} 1/ (\alpha_m/4^i + 1)}
\end{align} \else
\begin{align}\label{t_star}
    4^i K = \sum_{m=1}^{M} \sum_{k=1}^{K} X^\star_{mk} = \sum_{m=1}^{M} \frac{t^\star}{ (\alpha_m/4^i + 1)} ~=~ t^\star \sum_{m=1}^{M} \frac{1}{(\alpha_m/4^i + 1) }
    ~~\Rightarrow~~ t^\star ~=~ \frac{4^i K}{\sum_{m=1}^{M} 1/ (\alpha_m/4^i + 1)}
\end{align}\fi which justifies  \eqref{tau}.

\paragraph{Observation} Note that the solution of the relaxed LP (\ref{lp:formulation}) can be directly used for scheduling of actions by adding $\max{(2\alpha_{M-1}, \alpha_m )}$ to the end time $t^\star$. Since the relaxation in general does not give a feasible solution for the ILP, we add $\max{(2\alpha_{M-1}, \alpha_M)}$ to the end time of the relaxed ILP to guarantee a feasible solution for the ILP.
%\textcolor{violet}{(we will add in the paper in more detail why $\max{(2\alpha_{M-1}, \alpha_M)}$ extra pulls are necessary)}. 
As the additional time slots accumulate regret across all agents, this can result in $\Omega(M\alpha_M)$ additional regret which can be large for large $M$. Our algorithm improves the $M$ factor in $M\alpha_M$.

\section{MISSING PROOFS}
\label{app:missing-proofs}

\begin{table*}[tbhp!]
\centering
\caption{Notation} \label{table:notation}
\begin{tabular}{lcl}
%  &  & \\
\toprule
$4^i$& : & Number of effective pulls in batch $i$ for each active action \\
$\gA$& : & Set of actions, $|\gA| = K$  \\
$\gA_i$& : & Set of active actions in batch $i$, $|\gA_i| = K^{(i)}$\\
$\alpha_m$& : & $= \lceil 4 \log{T} / \log{(1/\epsilon_m)}\rceil-1$, number of repetitions for agent $m$\\
$\Delta_a$& : & $= \max_{a' \in \gA} \mu_{a'} - \mu_a$, suboptimality gap for action $a$\\
$G$& : & The event that at least one instruction among the times $t,t+1,\cdots,t+\alpha_m-1$ will not be\\
&  & erased for all agents $m$ and all times $t$\\
$G_i'$& : & $ = \left\{ | \evmu^{(j)}_a - \evmu_a| ~\leq~ 2 \sqrt{\frac{\log{(KMT)}}{2 \cdot 4^j}}  ~~\forall a \in \gA_j,~ j \in [i-1] \right\}$, the event that empirical means of\\ 
&  &active actions in batch $j$ ($\forall a \in A_j$) is in confidence region for all batches until batch $i$\\
$M$& : & Number of agents \\
$\mu_a$& : & Reward mean of action $a$\\
$\mu^{(i)}_a$& : & The empirical mean calculated for action $a$ at batch $i$ (as defined in step~\ref{step:emp-mean} in Algorithm~\ref{main})\\
$N_1^{(i)}$& : & $=\frac{M}{\sum\limits_{m=1}^{M} 1 / (\alpha_m + 4^i)}$, a term that appears in regret\\
$N_2^{(i)}$& : &$=12 \cdot 4^i$, a term that appears in regret \\
$R_T$& : & Regret of $K$ arm bandit over $M$ channels with horizon $T$\\
$R^{(i)}_T$& : & Regret of batch $i$ for $K$ arm bandit over $M$ channels with horizon $T$\\
$T^{(i)}$& : & Length of the scheduling outputted by \Algref{scheduling-alg} for batch $i$ \\
$T_i$& : & The total number of instructions played by all agents due to instructions sent in batch $i$ \\
$T_{ia}$& : & Number of times action $a$ is played by agents due to an instruction sent in batch $i$ \\
$\hat{K}$& : & Number of actions unassigned in the first part of the scheduling (as described in \Algref{scheduling-alg} line \ref{schedalg:Khat})\\
\bottomrule
\end{tabular}
\end{table*}

\subsection{Proof of Lemma \ref{lem:schedule-endtime}}
\label{app:proof-lemma-1}
In this section, we present the detailed proof of Lemma \ref{lem:schedule-endtime}. \\

\lemmasched*

We prove the upper bound on the end time in two steps.\\ 
\textbf{Step A.} First, we claim that the algorithm uses the first $4^i K \tau$ rounds to schedule all $4^i$ pulls of at least $(K-M)^{+}$ actions: \\ 
Each agent $m$ takes $\alpha_m + 4^i$ to complete all pulls of an action; hence, it can play all pulls of at least
\[
    \left\lfloor \frac{4^i K \tau}{\alpha_m + 4^i} \right\rfloor
\] actions. Hence, the total number of actions scheduled across all channels during the first $4^i K \tau$ rounds is
\begin{equation*}
\begin{aligned}
    \sum\limits_{m=1}^{M} \left\lfloor \frac{4^i K \tau}{\alpha_m + 4^i} \right\rfloor ~\geq~ \sum\limits_{m=1}^{M} \left( \frac{4^i K \tau}{\alpha_m + 4^i} - 1 \right) ~=~ K\tau \sum\limits_{m=1}^{M} \frac{1}{\alpha_m/4^i + 1} - M ~=~ K-M.
\end{aligned}
\end{equation*}
A lower bound of $(K-M)^+$ follows by the non-negativity of the number of scheduled pulls.\\
\textbf{Step B.} The second step is to show that the remaining number of actions $\hat{K} \leq K - (K-M)^{+} = \min{(K,M)}$ can be scheduled using an additional time of 
\[
    6 \left( \frac{\sum_{m=1}^{M} \alpha_m}{M} + 2\frac{4^i K}{M} \right).
\] Recall that Algorithm~\ref{scheduling-alg} divides the $4^i$ pulls of each of the remaining actions into \ifarxivFormat$\max{(1, \lfloor \frac{M}{2\hat{K}}}\rfloor)$ \else$\max{(1, \lfloor M / 2\hat{K}}\rfloor)$\fi equal parts and assign each part to an agent. Hence, each part will have number of pulls 
\begin{align}
    \frac{4^i}{\max{(1, \lfloor M / 2\hat{K}}\rfloor)} ~\overset{(a)}{\leq}~ \min{(4^i, \frac{4\hat{K}}{M} 4^i)} \label{eq:num_pulls_per_part}
\end{align}
and there will be at most $ M $ such parts. The first $\lfloor M / 2 \rfloor$ agents can be used for scheduling these parts in a way such that each agent is assigned at most three parts. It follows that each agent $m$ needs at most $3 \alpha_m + 3 \min{(4^i, \frac{4\hat{K}}{M} 4^i)}$ time to perform the scheduled pulls. Thus  the total number of rounds required to schedule the remaining pulls can be bounded by
\ifarxivFormat
\begin{align}
    3 \max_{m\in \{1,\cdots,\lfloor M/2 \rfloor\}}\alpha_m + 3 \min{(4^i, \frac{4\hat{K}}{M} 4^i)} &~\stackrel{(i)}{=}~ 3 \alpha_{\lfloor M/2 \rfloor} + 3 \min{(4^i, \frac{4\hat{K}}{M} 4^i)} \nonumber \\
    &~\stackrel{(ii)}{\leq}~ 6 \frac{\sum_{m=1}^{M} \alpha_m}{M} + 3 \min{(4^i, \frac{4\hat{K}}{M} 4^i)} \label{eq:endtime_second_part}
\end{align}
\else
\begin{align}
    3 \max_{m\in \{1,\cdots,\lfloor M/2 \rfloor\}}\alpha_m + 3 \min{(4^i, \frac{4\hat{K}}{M} 4^i)} &~\stackrel{(i)}{=}~ 3 \alpha_{\lfloor M/2 \rfloor} + 3 \min{(4^i, \frac{4\hat{K}}{M} 4^i)} ~\stackrel{(ii)}{\leq}~ 6 \frac{\sum_{m=1}^{M} \alpha_m}{M} + 3 \min{(4^i, \frac{4\hat{K}}{M} 4^i)} \label{eq:endtime_second_part}
\end{align}\fi
where $(i), (ii)$ follow from the fact that $\alpha_m$'s are ordered, i.e., $\alpha_1 \leq \alpha_2 \leq \cdots \leq \alpha_M$. Combining this with the result from \textbf{Step A}, we get that the end time needed to send all actions in batch $i$.

\subsection{Proof of Theorem 1}
\label{app:proof-thm-1}

%\theoremone*
\noindent{\textbf{\Theoref{main-thm}} \textit{
Consider a distributed multi-armed bandit setting  with $K$ actions and $M$ agents connected through heterogeneous erasure channels with erasure probabilities $\{ \epsilon_i\}_{i=1}^{M}$. If \algoname\ is run with horizon $T$, then the expected regret is,
    \begin{align*}
        \mathbb{E}[R_T] \leq c \Bigg( \Bigg. \sum_{a: \Delta_a > 0} \Big( \Big.  \frac{\log{(KMT)}}{\Delta_a} + \frac{M \log{(MT)}}{\sum\limits_{m=1}^{M} 1 / (\alpha_m + \frac{\log{(KMT)}}{\Delta_{a}})} \Big. \Big) + \sum_{m=1}^{M} \alpha_m \log{(MT)}  +  \log{(MT)} \Bigg. \Bigg)
    \end{align*}      
   where $\alpha_m = \lceil 4 \log{T} / \log{(1/\epsilon_m)}\rceil-1$ is the number of repetitions at agent $m$, $\Delta_a$ is the suboptimality gap for action $a$, and $c > 0$ a constant.}}

%\noindent{\textit{Proof of \Theoref{main-thm}.}
The regret bound is reached by bounding the number of batches a suboptimal arm can survive as a function of the suboptimality gap, conditioned on a good event that we specify later. This gives a bound on the maximum sub-optimality gap at each batch which in turn gives a bound on the regret using the bound on the batch length given in Lemma~\ref{lem:schedule-endtime}. 

Let $G$ be the event that for all agents $m$ and for all times $t$, at least one instruction among the times $t,t+1,\cdots,t+\alpha_m-1$ will not be erased. Hence, the event $G$ means that for any agent $m$, we cannot have $\alpha_m$ or more consecutive erasures. This implies that, conditioned on $G$, when an action $a$ is sent $\alpha_m + 4^i$ consecutive times by the learner to agent $m$, each of the last $4^i$ pulls will generate a reward from the distribution of action $a$. We call these last $4^i$ pulls, the effective pulls.  The probability of the compliment of $G$ can be bounded as
\begin{align}
\sP[G^c] \stackrel{(i)}{\leq} \sum_{m=1}^M \sum_{t=1}^T {\epsilon_m}^{\alpha_m} \stackrel{(ii)}{\leq} \sum_{m=1}^M \sum_{t=1}^T \frac{1}{T^4} \stackrel{(iii)}{\leq} \frac{1}{M T},
\end{align}
where $(i)$ follows by the union bound over all agents $m$ and times $t$, $(ii)$ uses \ifarxivFormat$\alpha_m = \lceil \frac{4 \log{T} }{ \log{(1/\epsilon_m)}} \rceil - 1$ \else$\alpha_m = \lceil 4 \log{T} / \log{(1/\epsilon_m)} \rceil - 1$\fi, and $(iii)$ follows from $M\leq T$.

Define an event $G'_i$ as
\begin{equation}
    G'_i = \left\{ | \evmu^{(j)}_a - \evmu_a| ~\leq~ 2 \sqrt{\frac{\log{(KMT)}}{2 \cdot 4^j}}  ~~\forall a \in \gA_j,~ j \in [i-1] \right\}, \nonumber
\end{equation}

where $\mu_a^{(j)}$ is the empirical mean calculated for action $a$ at batch $j$, as defined in step~\ref{step:emp-mean} in Algorithm~\ref{main}. By Hoeffding's inequality and the fact that rewards lie in $[0,1]$ almost surely, we have that $\sP [ G'_i | G] \geq 1 - 0.25 / {(MT)}$. Consequently, events $G$ and $G'_i$ happening together have a probability 
\begin{equation}\label{eq:GGi_high_prob}
    \sP [ G'_i \cap G] ~\geq~ (1-0.25 / (MT))^2 ~\geq~ 1 - 2 / (MT). 
\end{equation} %\violet{I changed this to $1 - 2 / (MT)$ from $1 - 1 / (MT)$, but I can also change the assumption for the equation above to $2M < T$ and get $\leq 0.25 / (MT)$ for Eq 9.}

We first bound the number of batches, a suboptimal arm can survive as a function of the suboptimality gap. Conditioned on $G \cap G'_{i+1} $  and the elimination criterion in Algorithm~\ref{main}, a sub-optimal action $a$ can survive getting eliminated in batch $i$ only if $4 \sqrt{\frac{\log{(KMT)}}{2 \cdot 4^i}} \geq \Delta_a / 2$.  This implies that $a$ can be in $\gA_{i+1}$ only when 
\begin{equation} \label{eq:bnd-elim-batch}
    i \leq \left\lceil \log_4{ \left( \frac{ 32 \log{(KMT)}}{\Delta_{a}^2}  \right)} \right\rceil,
\end{equation} i.e., whenever the batch number $i$ is greater than the bound provided in \eqref{eq:bnd-elim-batch}, $a \not\in \gA_i$. 

Using the result of Lemma~\ref{lem:schedule-endtime}, we know the number of sent instructions in each batch $i$ is upper bounded as
\begin{equation}\label{eq:n-pulls}
    M T^{(i)} ~\leq~ K^{(i)} M \cdot 4^i \tau + 6 \sum_{m=1}^{M} \alpha_m + 12 K^{(i)} 4^i,
\end{equation}
where $K^{(i)}=|\gA_i|$ is the number of actions at the start of batch $i$ and $T^{(i)}$ is the length of batch $i$. Conditioned on the event $G$ (we cannot have $\alpha_m$ consecutive erasures for any agent $m$), the last action played by agent $m$ in batch $i$ will be played at most $\alpha_m$ times in batch $i+1$ (due to potential erasures).
% \setlength{\tabcolsep}{10pt} 
% \begin{table*}[tbhp!]
% \centering
% \begin{threeparttable}
% \caption{Example of how an instruction from batch $i$ affects the next batch $i+1$. Notice that $t = \sum\limits_{j=1}^{i} T^{(j)}$ is the time learner sends the last instruction scheduled for batch $i$, hence, $t+1$ is the start time of batch $i+1$} \label{table:instruction_to_next_batch}
% \begin{tabular}{lcccccc}
% \textbf{Time}  & \textbf{$t=\sum\limits_{j=1}^{i} T^{(j)}$} & \textbf{$t+1$} & \textbf{$t+2$} & \textbf{$t+3$} & \textbf{...} & \textbf{$t+\alpha_m$} \\
% \toprule
% \textbf{Learner}         & $a_t^{(m)}$ & $a_{t+1}^{(m)}=a$ & $a_{t+2}^{(m)}=a$ & $a_{t+3}^{(m)}=a$ & $\cdots$ & $a_{t+\alpha_m}^{(m)}=a$\\
% \midrule
% \textbf{Agent m} &$\Tilde{a}_{t}^{(m)}=a'$ & $\Tilde{a}_{t+1}^{(m)}$ & $\Tilde{a}_{t+2}^{(m)}$ & $\Tilde{a}_{t+3}^{(m)}$ & $\cdots$ & $\Tilde{a}_{t+\alpha_m}^{(m)}$ \\
% \bottomrule
% \end{tabular}
% \end{threeparttable}
% \end{table*}
This implies that the total number of instructions, $T_i$, played by all agents due to instructions sent in batch $i$, can be bounded as 
\begin{equation}
T_i ~\leq~ \sum_{m=1}^{M} (T^{(i)} + \alpha_m) ~\leq~ K^{(i)}M \cdot 4^i \tau + 7  \sum_{m=1}^{M} \alpha_m + 12K^{(i)} 4^i .
\end{equation}

We utilize the following proposition, restated and proved at the end of \secref{app:proof-thm-1}, to bound the expected number of times a certain action is played due to an instruction sent in batch $i$.

\begin{restatable}{proposition}{propositionone}
 Conditioned on $(G\cap G'_i, \mathcal{A}_i)$, the expected number of times arm $a$ is played due to an instruction sent in batch $i$ is the same for all $a\in \mathcal{A}_i$. In particular, $\mathbb{E}[T_{ia}|G\cap G'_i,\mathcal{A}_i ]=\mathbb{E}[T_{ia'}|G\cap G'_i, \mathcal{A}_i], \quad  \forall a,a'\in \mathcal{A}_i$.
\end{restatable}

Conditioning on $\mathcal{A}_i$ in the previous proposition and in the following abbreviates conditioning on the event that the random set of surving actions in batch $i$ takes the value $\mathcal{A}_i$.

% \textcolor{cyan}{Perhaps say something like "for convenience, we denote the event that $a \in \mathcal{A}_i$  simply by $\mathcal{A}_i$ } {\color{blue} [By $\mathcal{A}_i$ we meant the set of surviving actions in batch $i$. We condition on $\mathcal{A}_i$ because it is a random set. Should we mention this here? Could you please let us know if there is a mistake or something that does not make sense for considering $\mathcal{A}_i$ as the set of surviving actions?]}

Then, we have that
\begin{align}\label{eq:n-pulls-per-arm}
    \mathbb{E}[T_{ia} | G\cap G'_i,\gA_i] ~=~ \frac{\mathbb{E}[T_{i} | G\cap G'_i, \gA_i]}{K^{(i)}} ~\leq~ M \cdot 4^i \tau + 7  \frac{\sum_{m=1}^{M} \alpha_m}{K^{(i)}} + 12 \cdot 4^i\ \ ~\forall a \in \mathcal{A}_i. 
\end{align}

Let $R_T^{(i)}$ be the regret of batch $i$. The regret of the algorithm can be bounded as
\ifarxivFormat
\begin{align}\label{eq:sep-reg}
    \mathbb{E}[R_T] &~=~ \sum\limits_{i=1}^{\log{(MT)}} \mathbb{E}[ R_T^{(i)}] ~\leq~ \sum\limits_{i=1}^{\log{(MT)}} \Big( \Big. \mathbb{E}[R_T^{(i)} |G \cap G'_{i}] + MT (1-\mathbb{P}[G \cap G'_{i}]) \Big. \Big) \nonumber \\
    &~\stackrel{(a)}{\leq}~ \sum\limits_{i=1}^{\log{(MT)}} (\mathbb{E}[\mathbb{E}[R_T^{(i)}|G \cap G'_{i}, \gA_i]] + 1) \nonumber \\
    &~=~ \sum\limits_{i=1}^{\log{(MT)}} \mathbb{E} [ \sum_a \mathbb{E}[T_{ia}|G \cap G'_{i}, \gA_i] \Delta_a ] + \log{(MT)} \nonumber \\
    &~\stackrel{(b)}{\leq}~ \sum\limits_{i=1}^{\log{(MT)}} \Bigg( \Bigg. \mathbb{E}[ \sum_a (N_1^{(i)}+N_2^{(i)}) \mathbb{E}[\mathds{1}[a\in \gA_i]|G \cap G'_{i}] \Delta_a] \nonumber \\
    & \qquad \qquad \qquad + \mathbb{E} [\sum_a 7 \sum_{m=1}^{M} \frac{\alpha_m}{K^{(i)}} \mathbb{E}[\mathds{1}[a\in \gA_i]|G \cap G'_{i}, \gA_i] \Delta_a ] \Bigg. \Bigg) + \log{(MT)} \nonumber \\
    &~\leq~ \sum\limits_{i=1}^{\log{(MT)}} \sum_a (N_1^{(i)}+N_2^{(i)}) \mathbb{E}[\mathds{1}[a\in \gA_i]|G \cap G'_{i}] \Delta_a + \mathbb{E} [7 \sum_{m=1}^{M} \alpha_m ] + \log{(MT)} \nonumber \\
    &~\leq~ \sum\limits_{i=1}^{\log{(MT)}} \sum_a (N_1^{(i)}+N_2^{(i)}) \mathbb{E}[\mathds{1}[a\in \gA_i]|G \cap G'_{i}] \Delta_a + c'' \log{(MT)} \sum_{m=1}^{M} \alpha_m + \log{(MT)},
\end{align}
\else
\begin{align}\label{eq:sep-reg}
    \mathbb{E}[R_T] &~=~ \sum\limits_{i=1}^{\log{(MT)}} \mathbb{E}[ R_T^{(i)}] ~\leq~ \sum\limits_{i=1}^{\log{(MT)}} \Big( \Big. \mathbb{E}[R_T^{(i)} |G \cap G'_{i}] + MT (1-\mathbb{P}[G \cap G'_{i}]) \Big. \Big) \nonumber \\
    &~\stackrel{(a)}{\leq}~ \sum\limits_{i=1}^{\log{(MT)}} (\mathbb{E}[\mathbb{E}[R_T^{(i)}|G \cap G'_{i}, \gA_i]] + 1) ~=~ \sum\limits_{i=1}^{\log{(MT)}} \mathbb{E} [ \sum_a \mathbb{E}[T_{ia}|G \cap G'_{i}, \gA_i] \Delta_a ] + \log{(MT)} \nonumber \\
    &~\stackrel{(b)}{\leq}~ \sum\limits_{i=1}^{\log{(MT)}} \Bigg( \Bigg. \mathbb{E}[ \sum_a (N_1^{(i)}+N_2^{(i)}) \mathbb{E}[\mathds{1}[a\in \gA_i]|G \cap G'_{i}] \Delta_a] \nonumber \\
    & & \mathllap{+ \mathbb{E} [\sum_a 7 \sum_{m=1}^{M} \frac{\alpha_m}{K^{(i)}} \mathbb{E}[\mathds{1}[a\in \gA_i]|G \cap G'_{i}, \gA_i] \Delta_a ] \Bigg. \Bigg) + \log{(MT)}} \nonumber \\
    &~\leq~ \sum\limits_{i=1}^{\log{(MT)}} \sum_a (N_1^{(i)}+N_2^{(i)}) \mathbb{E}[\mathds{1}[a\in \gA_i]|G \cap G'_{i}] \Delta_a + \mathbb{E} [7 \sum_{m=1}^{M} \alpha_m ] + \log{(MT)} \nonumber \\
    &~\leq~ \sum\limits_{i=1}^{\log{(MT)}} \sum_a (N_1^{(i)}+N_2^{(i)}) \mathbb{E}[\mathds{1}[a\in \gA_i]|G \cap G'_{i}] \Delta_a + c'' \log{(MT)} \sum_{m=1}^{M} \alpha_m + \log{(MT)},
\end{align}\fi
where $(a)$ follows from law of total expectation and \eqref{eq:GGi_high_prob}, $(b)$ follows from \eqref{eq:n-pulls-per-arm} and we use 
 $N_1^{(i)}= \frac{M}{\sum\limits_{m=1}^{M} 1 / (\alpha_m + 4^i)}$ and $N_2^{(i)}=12 \cdot 4^i$ for these quantities that do not depend on $\mathcal{A}_i$. We will bound each term in \eqref{eq:sep-reg} separately to get the final regret bound. 

We start by bounding the effect of the first term in~\eqref{eq:sep-reg}, $N_1^{(i)}=\frac{M}{\sum\limits_{m=1}^{M} 1 / (\alpha_m + 4^i)}$, on the final regret bound. We have that 
\begin{align}\label{eq:bnd-1}
    \sum\limits_{i=1}^{\log{(MT)}} \sum_a N_1^{(i)} \mathbb{E}[\mathds{1}[a\in \gA_i]|G \cap G'_{i}] \Delta_a &~=~ \sum\limits_{a} \sum\limits_{i=1}^{\log {(MT)}} \Delta_{a} \frac{M\mathbb{E}[\mathds{1}[a\in \gA_i]|G\cap G'_i]}{\sum\limits_{m=1}^{M} 1 / (\alpha_m + 4^i)} \nonumber \\
    &~\stackrel{(a)}{\leq}~ c \sum\limits_{a: \Delta_a > 0} \frac{M \log{(MT)}}{\sum\limits_{m=1}^{M} 1 / (\alpha_m + \frac{\log{(KMT)}}{\Delta_{a}})}
\end{align}
where $c$ is a universal constant, and $(a)$ follows from \eqref{eq:bnd-elim-batch} and the bound being an increasing function of $i$.

The effect of the second term in~\eqref{eq:sep-reg}, $N_2^{(i)}=12 \cdot 4^i$, 
\ifarxivFormat
\begin{align}\label{eq:bnd-3}
    \sum_a \sum\limits_{i=1}^{\log{(MT)}} N_2^{(i)} \mathbb{E}[\mathds{1}[a\in \gA_i]|G \cap G'_{i}] \Delta_a &~=~ 12 \sum\limits_{a} \sum\limits_{i=1}^{\left\lceil \log_4{ \left( \frac{ 32 \log{(KMT)}}{\Delta_{a}^2}  \right)} \right\rceil} 4^i \Delta_{a} \nonumber \\ &~\stackrel{(a)}{\leq}~ c' \sum_{a: \Delta_a > 0} \frac{\log{(KMT)}}{\Delta_a},
\end{align}
\else
\begin{align}\label{eq:bnd-3}
    & \sum_a \sum\limits_{i=1}^{\log{(MT)}} N_2^{(i)} \mathbb{E}[\mathds{1}[a\in \gA_i]|G \cap G'_{i}] \Delta_a ~=~ 12 \sum\limits_{a} \sum\limits_{i=1}^{\left\lceil \log_4{ \left( \frac{ 32 \log{(KMT)}}{\Delta_{a}^2}  \right)} \right\rceil} 4^i \Delta_{a} ~\stackrel{(a)}{\leq}~ c' \sum_{a: \Delta_a > 0} \frac{\log{(KMT)}}{\Delta_a}, 
\end{align}
\fi where $(a)$ follows from \eqref{eq:bnd-elim-batch}, and $c'$ is a universal constant. The final result follows by summing the bounds in \eqref{eq:bnd-1} and \eqref{eq:bnd-3}.

\propositionone*
\textit{Proof.} Recall that $T_{ia}$ is the number of times an agent plays arm $a$ due to an instruction sent in batch $i$.
We represent the schedule by the set $S = \{ \{ S_{mt} \}_{m=1}^{M} \}_{t=1}^{T^{(i)}}$, where $S_{mt}$ is the action the learner sends to agent $m$ at time $t$. Let $S(a\leftrightarrow a')$ represents the schedule where actions $a,a'$ are exchanged in the schedule $S$, i.e., $S(a\leftrightarrow a')_{mt}=a$ whenever $S_{mt}=a'$, $S(a\leftrightarrow a')_{mt}=a'$ whenever $S_{mt}=a$, otherwise $S(a\leftrightarrow a')_{mt}=S_{mt}$. We notice that conditioned on the schedule $S$ in batch $i$, whether an action is played in slot $t$ due to an instruction sent in batch $i$ is only a function of the erasures in batches $i,i+1,..$. Hence, we have that
\ifarxivFormat
\begin{align}
\mathbb{E}[T_{ia} | G \cap G_i', \mathcal{A}_i] &=~ \sum\limits_{S \in \mathbb{S}} \mathbb{P}[S | G \cap G_i', \mathcal{A}_i] \mathbb{E}[ T_{ia} | G \cap G_i',\mathcal{A}_i, S] =~ \sum\limits_{S \in \mathbb{S}} \mathbb{P}[S |\mathcal{A}_i] \mathbb{E}[ T_{ia} | G,S]\nonumber \\
&\stackrel{(a)}{=} \sum\limits_{S \in \mathbb{S}} \frac{1}{|\mathbb{S}|} \mathbb{E}[ T_{ia} |G, S] = \sum\limits_{S \in \mathbb{S}} \frac{1}{|\mathbb{S}|} \mathbb{E}[ T_{ia'} | G, S(a\leftrightarrow a')] = \sum\limits_{S \in \mathbb{S}} \frac{1}{|\mathbb{S}|} \mathbb{E}[ T_{ia'} | G, S] \nonumber \\ &=~ \mathbb{E}[T_{ia'} | G \cap G_i', \mathcal{A}_i],
\end{align}
\else
\begin{align}
\mathbb{E}[T_{ia} | G \cap G_i', \mathcal{A}_i] &=~ \sum\limits_{S \in \mathbb{S}} \mathbb{P}[S | G \cap G_i', \mathcal{A}_i] \mathbb{E}[ T_{ia} | G \cap G_i',\mathcal{A}_i, S] =~ \sum\limits_{S \in \mathbb{S}} \mathbb{P}[S |\mathcal{A}_i] \mathbb{E}[ T_{ia} | G,S]\nonumber \\
&\stackrel{(a)}{=} \sum\limits_{S \in \mathbb{S}} \frac{1}{|\mathbb{S}|} \mathbb{E}[ T_{ia} |G, S] = \sum\limits_{S \in \mathbb{S}} \frac{1}{|\mathbb{S}|} \mathbb{E}[ T_{ia'} | G, S(a\leftrightarrow a')] = \sum\limits_{S \in \mathbb{S}} \frac{1}{|\mathbb{S}|} \mathbb{E}[ T_{ia'} | G, S] =~ \mathbb{E}[T_{ia'} | G \cap G_i', \mathcal{A}_i],
\end{align}
\fi where $\mathbb{S}$ is the set of all (non-zero probability) possible schedules for batch $i$, and $(a)$ follows since the randomization in Algorithm~\ref{scheduling-alg} makes all the schedules in $\mathbb{S}$ equally probable.

\subsection{Proof of Theorem 2}
\label{app:proof-thm-2}

%\theoremtwo*
\noindent{\textbf{\Theoref{instance-indep-thm}} \textit{Consider the distributed multi-armed bandit setting with $K$ actions and $M$ agents connected through heterogeneous erasure channels $\{ \epsilon_i\}_{i=1}^{M}$. If \algoname is run for horizon $T$, then the expected regret is
    \begin{align*}
        R_T \leq c \Bigg( \Bigg. M \sqrt{\frac{ K T \log{(MT)} }{\sum_{m=1}^{M} 1 / (\alpha_m\Delta_{\star} + \log{(KMT)})}} ~ + \sum_{m=1}^{M} \alpha_m \log{(KMT)}\Bigg. \Bigg)
    \end{align*}      
   where $\Delta_{\star}$ is the value satisfying \[
    \Delta_{\star} = \frac{c' K \log{(MT)}}{T \sum\limits_{m=1}^{M} 1 / (\alpha_m + \frac{\log{(KMT)}}{\Delta_{\star}})},
   \] which can be efficiently approximated using the bisection method, $\alpha_m = \lceil 4 \log{T} / \log{(1/\epsilon_m)}\rceil -1$ number of repetitions and $c, c' > 0$ constants.}}

\noindent{\textit{Proof of \Theoref{instance-indep-thm}.}
From \eqref{eq:sep-reg}, the expected regret can be bounded as
\ifarxivFormat
\begin{align}\label{eq:ub_on_regret}
    \mathbb{E}[R_T]&~\leq~ \sum\limits_{i=1}^{\log{(MT)}} \sum_a \mathbb{E}[T_{ia}|G \cap G'_{i}] \Delta_a + \log{(MT)}\nonumber \\
    &~\leq~ MT \Delta + \sum\limits_{i=1}^{\log{(MT)}} \sum_{a:\Delta_a>\Delta} \mathbb{E}[T_{ia}|G \cap G'_{i}] \Delta_a + \log{(MT)} \nonumber \\
    &~\stackrel{(a)}{\leq}~ MT \Delta + \sum\limits_{i=1}^{\log{(MT)}} \sum_{a:\Delta_a>\Delta} (N_1^{(i)}+N_2^{(i)}) \mathds{1}[a\in \gA_i] \Delta_a + c''' \log{(MT)} \sum_{m=1}^{M} \alpha_m + \log{(MT)} \nonumber \\
    & ~\stackrel{(b)}{\leq}~ MT \Delta + c \sum\limits_{a: \Delta_a > \Delta} \left( \frac{M \log{(MT)}}{\sum\limits_{m=1}^{M} 1 / (\alpha_m + \frac{\log{(KMT)}}{\Delta_{a}})} + \frac{\log{(KMT)}}{\Delta_a} \right) + f(M, T, \valpha) \nonumber \\
    & ~\stackrel{(c)}{\leq}~ MT \Delta + c \sum\limits_{a: \Delta_a > \Delta}  \frac{2 M \log{(MT)}}{\sum\limits_{m=1}^{M} 1 / (\alpha_m + \frac{\log{(KMT)}}{\Delta_{a}})} + f(M, T, \valpha) \nonumber \\
    & ~\stackrel{(d)}{=}~ MT \Delta + \frac{c' K M \log{(MT)}}{\sum\limits_{m=1}^{M} 1 / (\alpha_m + \frac{\log{(KMT)}}{\Delta})} + f(M, T, \valpha) \nonumber \\
    &~\leq~ 2 \max{\left\{ TM \Delta, \frac{c' K M  \log{(MT)}}{\sum\limits_{m=1}^{M} 1 / (\alpha_m + \frac{\log{(KMT)}}{\Delta})} \right\}} + f(M, T, \valpha) ~~\forall \Delta > 0 
\end{align}
\else
\begin{align}\label{eq:ub_on_regret}
    \mathbb{E}[R_T]&~\leq~ \sum\limits_{i=1}^{\log{(MT)}} \sum_a \mathbb{E}[T_{ia}|G \cap G'_{i}] \Delta_a + \log{(MT)}\nonumber \\
    &~\leq~ MT \Delta + \sum\limits_{i=1}^{\log{(MT)}} \sum_{a:\Delta_a>\Delta} \mathbb{E}[T_{ia}|G \cap G'_{i}] \Delta_a + \log{(MT)} \nonumber \\
    &~\stackrel{(a)}{\leq}~ MT \Delta + \sum\limits_{i=1}^{\log{(MT)}} \sum_{a:\Delta_a>\Delta} (N_1^{(i)}+N_2^{(i)}) \mathds{1}[a\in \gA_i] \Delta_a + c''' \log{(MT)} \sum_{m=1}^{M} \alpha_m + \log{(MT)} \nonumber \\
    & ~\stackrel{(b)}{\leq}~ MT \Delta + c \sum\limits_{a: \Delta_a > \Delta} \left( \frac{M \log{(MT)}}{\sum\limits_{m=1}^{M} 1 / (\alpha_m + \frac{\log{(KMT)}}{\Delta_{a}})} + \frac{\log{(KMT)}}{\Delta_a} \right) + c''' \log{(MT)} \sum_{m=1}^{M} \alpha_m + \log{(MT)} \nonumber \\
    & ~\stackrel{(c)}{\leq}~ MT \Delta + c \sum\limits_{a: \Delta_a > \Delta}  \frac{2 M \log{(MT)}}{\sum\limits_{m=1}^{M} 1 / (\alpha_m + \frac{\log{(KMT)}}{\Delta_{a}})}  + c''' \log{(MT)} \sum_{m=1}^{M} \alpha_m + \log{(MT)} \nonumber \\
    & ~\stackrel{(d)}{=}~ MT \Delta + \frac{c' K M \log{(MT)}}{\sum\limits_{m=1}^{M} 1 / (\alpha_m + \frac{\log{(KMT)}}{\Delta})} + c''' \log{(MT)} \sum_{m=1}^{M} \alpha_m + \log{(MT)} \nonumber \\
    &~\leq~ 2 \max{\left\{ TM \Delta, \frac{c' K M  \log{(MT)}}{\sum\limits_{m=1}^{M} 1 / (\alpha_m + \frac{\log{(KMT)}}{\Delta})} \right\}} + c''' \log{(MT)} \sum_{m=1}^{M} \alpha_m + \log{(MT)} ~~\forall \Delta > 0 
\end{align}\fi where \ifarxivFormat $f(M, T, \valpha) = c''' \log{(MT)} \sum_{m=1}^{M} \alpha_m + \log{(MT)}$  and \else \fi$c, c', c''' > 0$ some constants. (a) follows from \eqref{eq:n-pulls-per-arm} where $N_1^{(i)}=M/(\sum_{m=1}^{M} 1 / (\alpha_m + 4^i))$ and $N_2^{(i)}=12 \cdot 4^i$. (b) follows from directly substituting \eqref{eq:bnd-1} and \eqref{eq:bnd-3} for the terms; and (c) follows from the fact that the first term is an increasing function of $\alpha_m$'s; therefore, 
$$\frac{M \log{(MT)}}{\sum\limits_{m=1}^{M} 1 / (\alpha_m + \frac{\log{(KMT)}}{\Delta_{a}})} ~\geq~ \frac{M \log{(MT)}}{\sum\limits_{m=1}^{M} 1 / \frac{\log{(KMT)}}{\Delta_{a}}} ~\geq~ \frac{\log{(KMT)}}{\Delta_a} ~~~\forall \{ \alpha_m\}_{m=1}^{M} \geq 0 . $$ (d) follows from the term inside the summation being a decreasing function of $\Delta_a$.

We choose $\Delta$ to be the value that minimizes the bound. Hence the optimal value $\Delta_{\star}$ satisfies:
\begin{align}
    TM \Delta_{\star} = \frac{c' K M \log{(MT)}}{\sum\limits_{m=1}^{M} 1 / (\alpha_m + \frac{\log{(KMT)}}{\Delta_{\star}})} \label{eq:optimal_delta}
\end{align}
Substituting \eqref{eq:optimal_delta} to the bound in \eqref{eq:ub_on_regret}, we get that
\begin{align}
    \mathbb{E}[R_T] & ~\leq~ 2 M \sqrt{ \frac{c' K T \log{(MT)}}{ \sum\limits_{m=1}^{M} 1 / (\alpha_m \Delta_{\star} + \log{(KMT)}) } } + c''' \log{(MT)} \sum_{m=1}^{M} \alpha_m + \log{(MT)}.
\end{align}
